# Supplementary material for: Text-driven Visual Synthesis with Latent Diffusion Prior
Source: arXiv:2302.08510 source file (2023-04-03)
Supplement: Supplementary file 1 [file fig_layered.tex]

\begin{figure*}
\centering

\mpage{0.02}{\raisebox{0pt}{\rotatebox{90}{}}}
\mpage{0.23}{{{\small{Input}}}}\hfill
\mpage{0.23}{{{\small{Text2LIVE~\cite{bar2022text2live}}}}}\hfill
\mpage{0.23}{{{\small{$L_{LSD}$ baseline}}}}\hfill
\mpage{0.23}{{{\small{Ours ($L_{FM} + L_{LSD} + L_{KL}$)}}}}\\

\vspace{1mm}

\mpage{0.02}{\raisebox{-10pt}{\rotatebox{90}{\small{horse \textrightarrow zebra}}}}
\mpage{0.23}{\frame{\includegraphics[width=\linewidth, trim=0 0 0 0, clip]{images/editing/supp/zebra/input.jpg}}}\hfill
\mpage{0.23}{\frame{\includegraphics[width=\linewidth, trim=0 0 0 0, clip]{images/editing/supp/zebra/text2live.png}}}\hfill
\mpage{0.23}{\frame{\includegraphics[width=\linewidth, trim=0 0 0 0, clip]{images/editing/supp/zebra/lsd.png}}}
\mpage{0.23}{\frame{\includegraphics[width=\linewidth, trim=0 0 0 0, clip]{images/editing/supp/zebra/lsd+fm+kl.png}}}\\

\vspace{1mm}

\mpage{0.02}{\raisebox{-10pt}{\rotatebox{90}{\small{bear \textrightarrow pandas}}}}
\mpage{0.23}{\frame{\includegraphics[width=\linewidth, trim=0 0 0 0, clip]{images/editing/supp/pandas/input.jpeg}}}\hfill
\mpage{0.23}{\frame{\includegraphics[width=\linewidth, trim=0 0 0 0, clip]{images/editing/supp/pandas/text2live.png}}}\hfill
\mpage{0.23}{\frame{\includegraphics[width=\linewidth, trim=0 0 0 0, clip]{images/editing/supp/pandas/lsd.png}}}
\mpage{0.23}{\frame{\includegraphics[width=\linewidth, trim=0 0 0 0, clip]{images/editing/supp/pandas/lsd+fm+kl.png}}}\\

\vspace{3mm}

% \mpage{0.02}{\raisebox{-10pt}{\rotatebox{90}{\small{bread\textrightarrow sandwich}}}}
% \mpage{0.31}{\frame{\includegraphics[width=\linewidth, trim=0 0 0 0, clip]{images/editing/bread/bread.jpeg}}}\hfill
% %\mpage{0.235}{\frame{\includegraphics[width=\linewidth, trim=0 0 0 0, clip]{images/editing/bread/text2live_sandwich.png}}}\hfill
% \mpage{0.31}{\frame{\includegraphics[width=\linewidth, trim=0 0 0 0, clip]{images/editing/bread/lr_wokl_sandwich.png}}}\hfill
% \mpage{0.31}{\frame{\includegraphics[width=\linewidth, trim=0 0 0 0, clip]{images/editing/bread/sandwich.png}}}\\

\caption{\textbf{Visual comparisons on layered image editing.}}
\label{fig:supp_comparison_layered_editing}
\end{figure*}
